# Supplementary material for: Unravelling coherences in the FMO complex
Source: arXiv:1709.00318 ancillary file (2017-10-13)
Supplement: Supplementary file 1 [file Thyrhaug_et_al_SI.pdf]

# Unravelling coherences in the Fenna-Matthews-Olson complex

## - Supplementary Information -

Erling Thyrhaug*[,1], Roel Tempelaar*[,2], Marcelo J. P. Alcocer[1], Karel Žídek†[,1], David Bína[3], Jasper Knoester[4], Thomas L. C. Jansen[4], and Donatas Zigmantas‡[,1]

[1]Department of Chemical Physics, Lund University, P.O. Box 124, 22100 Lund, Sweden

[2]Department of Chemistry, Columbia University, 3000 Broadway, New York, New York 10027, USA

[3]Biology Centre CAS, Branišovská 31, and Faculty of Science, University of South Bohemia, Branišovská 1760, 370 05 České Budějovice, Czech Republic

[4]University of Groningen, Zernike Institute for Advanced Materials, Nijenborgh 4, 9747AG Groningen, The Netherlands

# Contents

**1 Theoretical methods** **ii**

*These authors contributed equally to this work.

†Current address: TOPTEC, Institute of Plasma Physics, Academy of Sciences of the Czech Republic, Za Slovankou 1782/3, 182 00 Prague 8, Czech Republic

‡donatas.zigmantas@chemphys.lu.se

2 **Experimental and Theoretical Total Absorptive Spectra at** $t_2 = 40\text{fs}$ **v**

3 **Selected Experimental Rephasing Spectra** **vi**

4 **Selected Kinetic Traces and Fits** **vii**

5 **Additional Experimental Oscillation maps** **ix**

6 **Analysis of Selected Pathways** **x**

7 **Selection of Ground State Signals in DC experiments** **xi**

# 1 Theoretical methods

The model applied to simulate linear absorption and the all-parallel (AP) polarized 2D spectra is discussed in detail in Ref. 1. We will briefly reiterate the most important aspects, and then continue to outline the adaptations made to simulate the double-cross (DC) polarized 2D spectra.

The employed electronic Hamiltonian is based on earlier parametrizations of the Fenna-Matthews-Olson (FMO) complex from *Chlorobium tepidum* which consider 7 bacteriochlorophyl *a* (BChl) chromophores for each monomeric unit and neglect the small interactions between monomers.[2] The applied electronic couplings and BChl site energies are summarized in Tab. 1 of Ref. 1, and are obtained from fittings to linear absorption, circular dichroism, and triplet-minus-singlet spectra.[2]

For each BChl, coupling of electronic degrees of freedom to a single (undamped) vibrational mode is included explicitly in the Hamiltonian though the vibronic exciton model.[3] The vibrational quantum is taken to be $160\,\text{cm}^{-1}$ while the Huang-Rhys factor is set equal to 0.02 (Refs. 4,5, and 6). This vibration is described in the single-particle approximation[7,8] using the respective eigenbases for (unshifted) ground state and (shifted) excited state vibrational levels.

The remaining vibrational degrees of freedom are accounted for by coupling each BChl

site energy to (uncorrelated) over-damped Brownian oscillators,[9] each having an associated width of $75\,\mathrm{cm}^{-1}$ (Refs. 10 and 6) and a correlation time of 140 fs (Ref. 11).

The quantum dynamics is obtained through time-integration of the Schrödinger equation[12,13] using a 5 fs time resolution. A Trotter-inspired propagation scheme is employed in order to keep calculation costs manageable.[1,14] A further approximation taken for the sake of numerical efficiency is a neglect of feedback from the Brownian oscillators to the electronic degrees of freedom (high-temperature approximation), which instead of the fast down-hill energy transfer observed for FMO[15] results in equal quantum populations.[1]

The molecular transition dipole moments are taken to be constant (Condon approximation),[11] their values (summarized in Tab. 2 of Ref. 1) extracted from crystallographic data, RCSB Protein Data Bank, file 3ENI (Ref. 16).

Theoretical linear absorption shown in Fig. 1 is obtained through a Fourier transform of the time-dependent dipole-dipole correlation function,[9] slightly smoothed by multiplication with an exponential having a 1/e decay time of 5 ps, and taking an average over 50,000 (uncorrelated) Brownian oscillator trajectories (dynamics disorder).

2D spectra are calculated through evaluation of the 4-point dipole correlation functions,[9] smoothed using an exponential decay time of 5 ps. The light-pulses are assumed to be impulsive, which is justified by the narrow absorption lineshape of FMO as compared to the laser spectrum (see Fig. 1).

What is different from the way 2D spectra were calculated in Ref. 1 is the method used to describe the pulse polarizations. In Ref. 1, the molecular transition dipoles were taken as the frame of reference, and the isotropic distribution of complexes in the sample was accounted for by weighing all 21 combinations with which the (all-parallel polarized) pulses can interact with the dipoles.[1,17] Here, the frame of reference is shifted towards the laser pulses (effectively adopting a lab frame). Accordingly, only one set of laser pulses is evaluated per polarization sequence, while each complex in the sample is randomly rotated through the following procedure.[18] First, two three-dimensional column vectors, $\vec{u}$ and $\vec{v}$, are constructed by drawing their components independently from a normal distribution centered at 0. Vector

$\vec{u}$ is normalized and its component parallel to $\vec{u}$ is projected out according to $\vec{v} = \vec{v} - \vec{u}(\vec{u}' \cdot \vec{v})$. Upon normalization of $\vec{v}$, a third vector is generated through an outer product of $\vec{u}$ and $\vec{v}$, $\vec{w} = \vec{u} \times \vec{v}$. Subsequently, a unitary matrix is constructed as $U = [\vec{u}\ \vec{v}\ \vec{w}]$. Finally, each molecular dipole is transformed according to $\vec{\mu}_n \to U\vec{\mu}_n$. Upon averaging over randomly drawn vectors $\vec{u}$ and $\vec{v}$, an isotropic distribution of complexes is retained. The pulse polarizations are then described by simply adopting the associated polarization angles: $\langle 0°, 0°, 0°, 0° \rangle$ for all-parallel (AP) and $\langle 45°, -45°, 90°, 0° \rangle$ for double-cross (DC) polarizations. All 2D spectra have been averaged over a total of 250,000 realizations including random rotations and random Brownian oscillator trajectories.

## 2 Experimental and Theoretical Total Absorptive Spectra at $t_2 = 40$fs

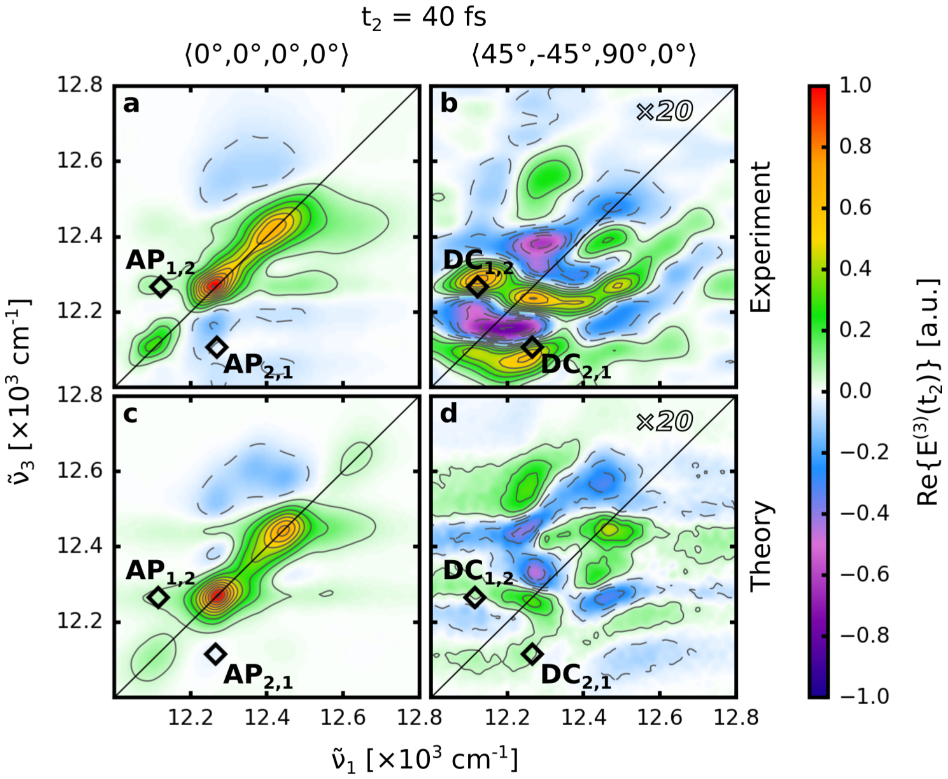


Figure 1: **Experimental and Theoretical Total Spectra at** 77 K**.** Real component of the total (rephasing + non-rephasing) 2D spectra at $t_2 = 40$fs. Experimental (**a, b**) and theoretical (**c, d**) spectra resulting from the all-parallel polarized pulse sequence (**a, c**) and the double-cross polarized pulse sequence (**b, d**) are shown. The spectra are normalised to the exciton 2 diagonal peak of the AP spectra and the DC spectra are scaled by a factor of 20 for clarity.

## 3 Selected Experimental Rephasing Spectra

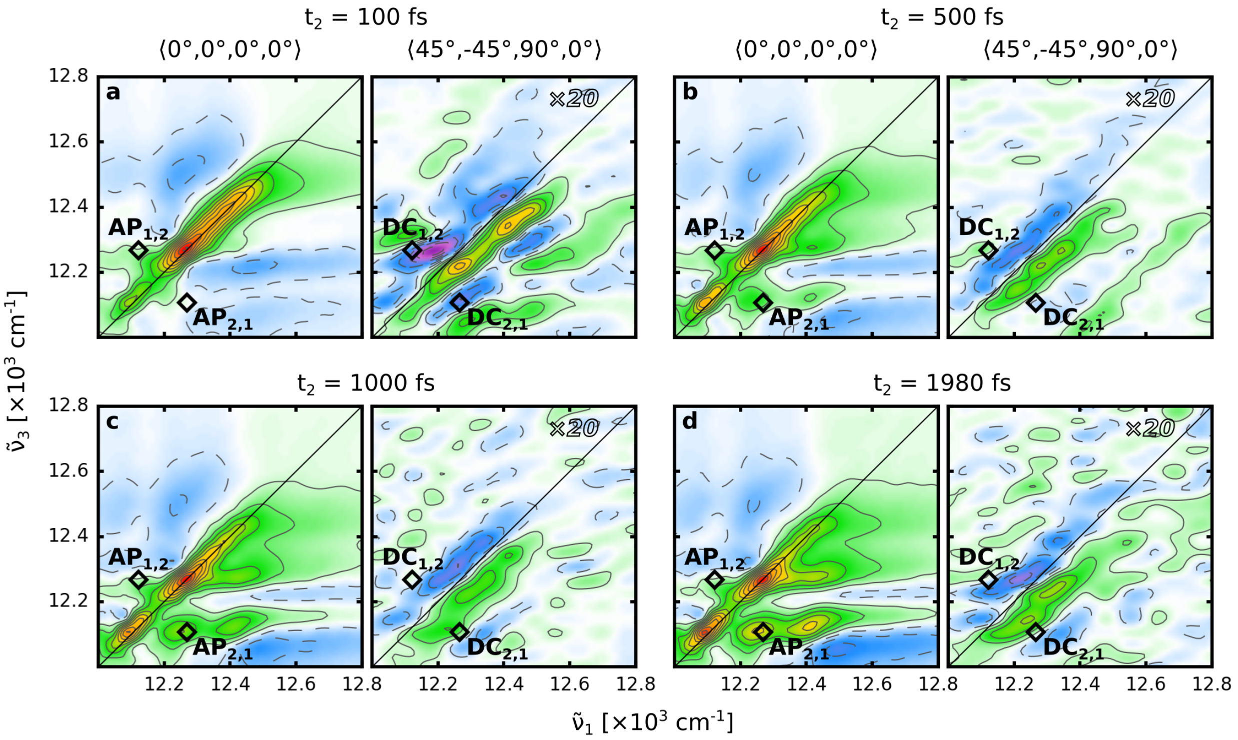


Figure 2: **Selected Experimental Rephasing Spectra.** Real component of the rephasing 2D spectra at $t_2 = 100, 500, 1000$ and 1980fs (**a**–**d** respectively). Experimental 2D spectra resulting from the all-parallel polarized pulse sequence (left columns) and the double-cross polarized pulse sequence (right columns) are shown. The spectra are normalised to the exciton 2 diagonal peak of the AP spectra and the DC spectra are scaled by a factor of 20 for clarity.

## 4 Selected Kinetic Traces and Fits

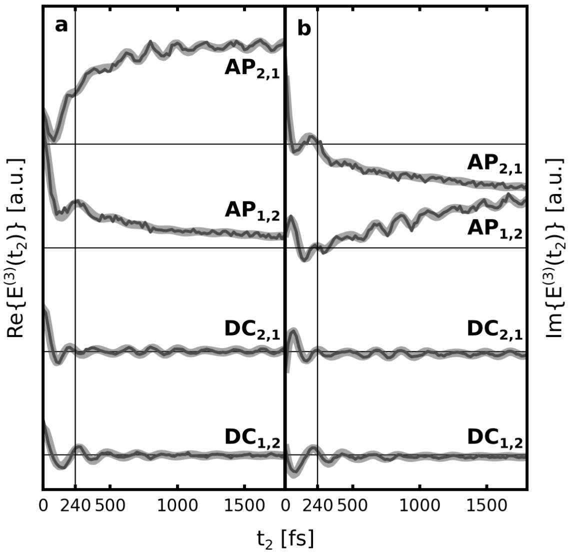


Figure 3: **Full fits of selected $t_2$ traces. (a)** Real and **(b)** imaginary components of experimental rephasing $t_2$ dynamics (black) at the cross-peak locations labelled in Fig. 1. Individual time-domain fits (grey) corresponding to Eq. 1 parameterised with the values in Tab. 1 are overlaid onto each trace. The traces are vertically offset for clarity.

| | $m$ | $A_m^{QB}$ | $\tau_m^{QB}$ | $\omega_m$ | $\phi_m$ | $n$ | $A_n^{Re}$ | $\tau_n^{Re}$ | $A_n^{Im}$ | $\tau_n^{Im}$ |
|---|---|---|---|---|---|---|---|---|---|---|
| | | [a.u.] | [fs] | [$2\pi c \cdot cm^{-1}$] | [rad] | | [a.u.] | [fs] | [a.u.] | [fs] |
| $AP_{2,1}$ | 1 | 1.48 | 150 | -96 | 0.61 | 1 | -5.71 | 300 | 1.71 | 244 |
| | 2 | 0.37 | 2090 | -166 | 0.14 | 2 | 0 | $\infty$ | -5.27 | 918 |
| | 3 | 0.29 | 1140 | -204 | 0.16 | 3 | 5.61 | $\infty$ | -2.40 | $\infty$ |
| $AP_{1,2}$ | 1 | 3.37 | 117 | 119 | 0.00 | 1 | 2.54 | 401 | 3.91 | 91 |
| | 2 | 0.07 | 1903 | 159 | 3.49 | 2 | 0.99 | 4009 | 2.72 | 1046 |
| | 3 | 0.07 | 2776 | 41 | 4.14 | 3 | 0.01 | $\infty$ | 2.94 | $\infty$ |
| $DC_{2,1}$ | 1 | 2.81 | 56 | -155 | 5.57 | 1 | -0.05 | 419 | 1.02 | 30 |
| | 2 | 0.24 | 1558 | -164 | 6.24 | 2 | 0.02 | $\infty$ | -0.13 | $\infty$ |
| | 3 | 0.08 | 2465 | -205 | 6.01 | – | – | – | – | – |
| $DC_{1,2}$ | 1 | 1.67 | 143 | 135 | 0.16 | 1 | -0.02 | $\infty$ | -0.09 | $\infty$ |
| | 2 | 0.27 | 691 | 164 | 2.43 | – | – | – | – | – |
| | 3 | 0.11 | 450 | 234 | 0.19 | – | – | – | – | – |

Table 1: **Fit parameters.** Parameterization of Eq. 1 for the time-domain fits presented in Fig. 3.

# 5 Additional Experimental Oscillation maps

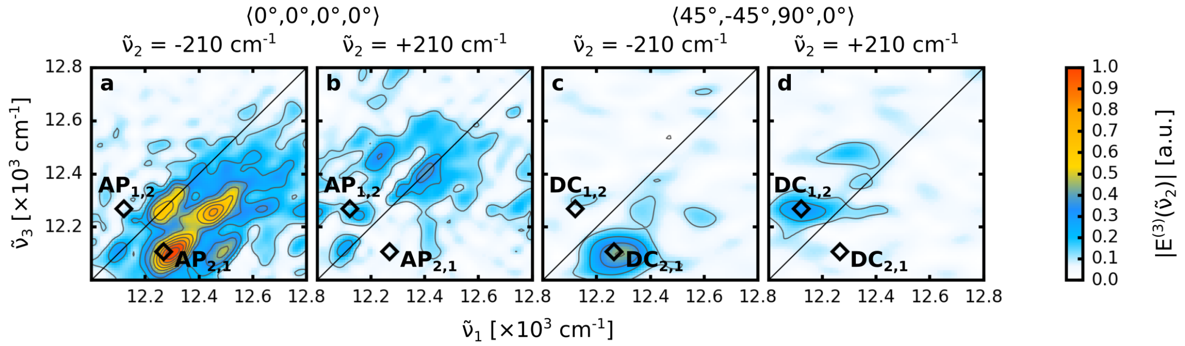


Figure 4: **Experimental $\pm 210\,\mathrm{cm}^{-1}$ oscillation maps.** Experimental Fourier amplitude maps at $\pm 210\,\mathrm{cm}^{-1}$ obtained by Fourier transformation of the 2D datasets along $t_2$ after subtraction of multi-exponential population dynamics. Maps with the all parallel (left, **a,b**) and double-cross (right, **c,d**) pulse sequences are shown. The maps are normalized to the experimental $\mathrm{AP}_{2,1}$ $-210\,\mathrm{cm}^{-1}$ amplitude.

# 6 Analysis of Selected Pathways

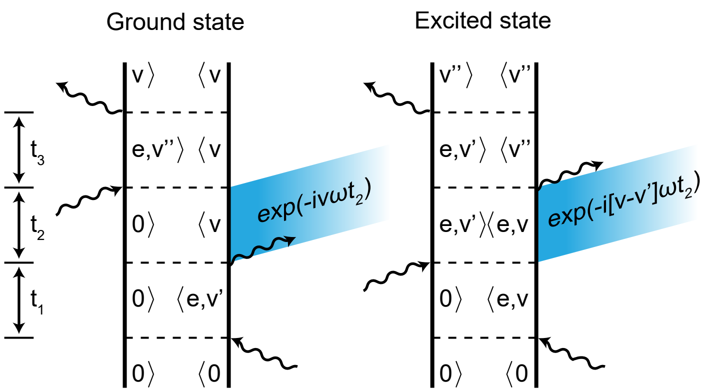


Figure 5: **Double-sided Feynman diagrams demonstrating that spectral oscillations recorded in the rephasing signal having a positive wavenumber can only originate from excited state coherences.** Shown on the left as a reference are the excitation, population, and detection time intervals, indicated as $t_1$, $t_2$, and $t_3$, respectively. The left diagram represents ground state bleach, whereas the right diagram depicts stimulated emission. The molecular system initiates in the vacuum state (0) in both cases. Interaction with the optical field (wiggling arrows) induces transition to and from some electronic excited state (e), while vibronic coupling mixes the vibrational state (v). For ground state bleach, coherence existing during the waiting time always involves a vibrationally excited ket (v) and an unexcited bra (0). Hence, such ground state coherence will always evolve as $e^{iv\omega t_2}$, with $\omega$ as the vibrational quantum, resulting in negative beat frequencies. For stimulated emission (and likewise for excited state absorption), the waiting time is preceeded by both ket and bra interactions, creating a coherence $|e, v'\rangle\langle e, v|$ that can have either a positive ($v > v'$) or a negative ($v < v'$) frequency. The diagrams adopt a single-molecule representation for the sake of clarity, however, the principle shown here does not alter for a coupled system.

# 7 Selection of Ground State Signals in DC experiments

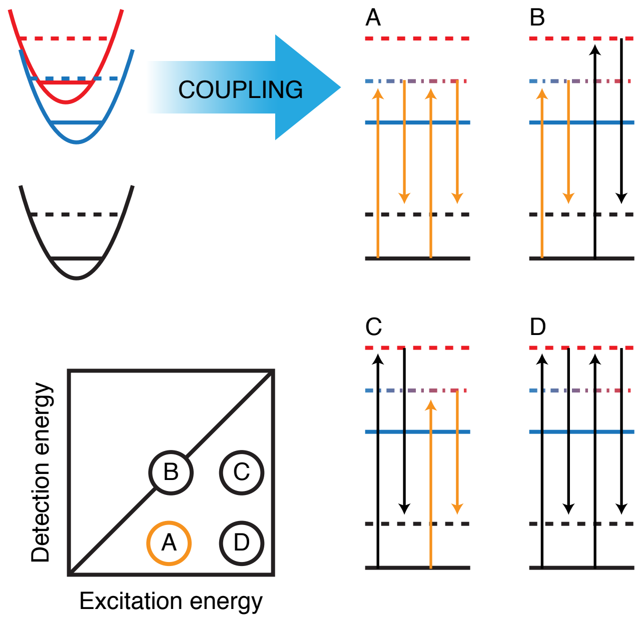


Figure 6: **Impact of pulse polarizations on Fourier transform amplitude peaks for the representative case of two pigments whose vibronic manifolds (red and blue parabolas) are offset by the vibrational quantum.** Upon electronic coupling, the resonance between the zero-phonon level of one pigment (solid red line) and the one-phonon level of the other (dashed blue line) results in a mixed level (red-blue dash-dotted line), while both pigments share the same ground state (black lines). Diagrams A-D show all possible rephasing ground state bleach pathways, where the arrows represent optical transitions. Transitions towards and from the mixed level (yellow arrows) involve the dipoles of both pigments, and can therefore be induced twice through a pair of perpendicularly polarized pulses. All other transitions (black arrows) only involve a single molecular dipole and will only survive the all-parallel pulse scheme. Hence, upon changing from an all-parallel to a cross-polarized sequence, the square of peaks shown in the schematic 2D plot will reduce to a single peak (A), whose underlying transitions all involve the mixed level.

# References

[1] Tempelaar, R., Jansen, T. L. C. & Knoester, J. Vibrational Beatings Conceal Evidence of Electronic Coherence in the FMO Light-Harvesting Complex. *J. Phys. Chem. B* **118**, 12865–12872 (2014).

[2] Vulto, S. I. E. *et al.* Exciton Simulations of Optical Spectra of the FMO Complex from the Green Sulfur Bacterium Chlorobium tepidum at 6 K. *J. Phys. Chem. B* **102**, 9577–9582 (1998).

[3] Holstein, T. Studies of polaron motion. *Ann. Phys.* **8**, 325–342 (1959).

[4] Rätsep, M. & Freiberg, A. Electronphonon and vibronic couplings in the FMO bacteriochlorophyll a antenna complex studied by difference fluorescence line narrowing. *J. Lumin.* **127**, 251–259 (2007).

[5] Tiwari, V., Peters, W. K. & Jonas, D. M. Electronic resonance with anticorrelated pigment vibrations drives photosynthetic energy transfer outside the adiabatic framework. *Proc. Natl. Acad. Sci. U.S.A* **110**, 1203–1208 (2013).

[6] Christensson, N., Kauffmann, H. F., Pullerits, T. & Mančal, T. Origin of Long-Lived Coherences in Light-Harvesting Complexes. *J. Phys. Chem. B* **116**, 7449–7454 (2012).

[7] Philpott, M. R. Theory of the Coupling of Electronic and Vibrational Excitations in Molecular Crystals and Helical Polymers. *J. Chem. Phys.* **55**, 2039–2054 (1971).

[8] Spano, F. C. Absorption and emission in oligo-phenylene vinylene nanoaggregates: The role of disorder and structural defects. *J. Chem. Phys.* **116**, 5877–5891 (2002).

[9] Mukamel, S. *Principles of Nonlinear Optical Spectroscopy* (Oxford University Press, 1995), 1 edn.

[10] Brixner, T. *et al.* Two-dimensional spectroscopy of electronic couplings in photosynthesis. *Nature* **434**, 625–628 (2005).

[11] Olbrich, C. *et al.* From Atomistic Modeling to Excitation Transfer and Two-Dimensional Spectra of the FMO Light-Harvesting Complex. *J. Phys. Chem. B* **115**, 8609–8621 (2011).

[12] Jansen, T. l. C. & Knoester, J. Nonadiabatic Effects in the Two-Dimensional Infrared Spectra of Peptides: Application to Alanine Dipeptide. *J. Phys. Chem. B* **110**, 22910–22916 (2006).

[13] Torii, H. Effects of Intermolecular Vibrational Coupling and Liquid Dynamics on the Polarized Raman and Two-Dimensional Infrared Spectral Profiles of Liquid N,N -Dimethylformamide Analyzed with a Time-Domain Computational Method. *J. Phys. Chem. A* **110**, 4822–4832 (2006).

[14] Liang, C. & Jansen, T. L. C. An Efficient N 3 -Scaling Propagation Scheme for Simulating Two-Dimensional Infrared and Visible Spectra. *J. Chem. Theory Comput.* **8**, 1706–1713 (2012).

[15] Thyrhaug, E., Žídek, K., Dostál, J., Bína, D. & Zigmantas, D. Exciton Structure and Energy Transfer in the FennaMatthewsOlson Complex. *J. Phys. Chem. Lett.* **7**, 1653–1660 (2016).

[16] Tronrud, D. E., Wen, J., Gay, L. & Blankenship, R. E. The structural basis for the difference in absorbance spectra for the FMO antenna protein from various green sulfur bacteria. *Photosynth. Res.* **100**, 79–87 (2009).

[17] Hochstrasser, R. M. Two-dimensional IR-spectroscopy: polarization anisotropy effects. *Chem. Phys.* **266**, 273–284 (2001).

[18] Brannon, R. M. *Rotation: A review of useful theorems involving proper orthogonal matrices referenced to three-dimensional physical space* (Retreived from http://www.mech.utah.edu/˜brannon/public/rotation.pdf, 2002).
